# Supplementary material for: Vision-language models for decoding provider attention during neonatal resuscitation
Source: arXiv:2404.01207 source file (2024-04-01)
Supplement: Supplementary file 1 [file 6_suppl.tex]

\clearpage
\setcounter{page}{1}
\maketitlesupplementary
